# Supplementary material for: Saving Critical Nodes with Firefighters is FPT
Source: arXiv:1705.10923 source file (2017-05-31)
Supplement: Supplementary file 1 [file ffcs-appendix.tex]

\subsection*{NP-hardness}

In this section, we state the proof of Theorem 13.

\subsection*{No Polynomial Kernel}

In this section, we state the proof of Theorem 28.
